# Supplementary material for: MIRA: Multimodal Iterative Reasoning Agent for Image Editing
Source: arXiv:2511.21087 source file (2026-02-25)
Supplement: Supplementary file 1 [file supplementary.tex]

\clearpage
\begin{figure*}[htbp]
  \centering
   \includegraphics[width=\textwidth]{fig/qual_supp1.png}

   \caption{Qualitative comparison of MIRA against leading proprietary and open-source image editing models on complex instructions.}
   \label{fig:qual_supp1}
\end{figure*}

\begin{figure*}[htbp]
  \centering
   \includegraphics[width=\textwidth]{fig/qual_supp2.png}

   \caption{Qualitative comparison of MIRA against leading proprietary and open-source image editing models on complex instructions.}
   \label{fig:qual_supp2}
\end{figure*}
